# Supplementary material for: Inferring simple but precise quantitative models of human oocyte and early embryo development
Source: arXiv:2103.12187 source file (2021-03-22)
Supplement: Supplementary file 1 [file si.pdf]

# 1 Inference and Regression Methods

## 1.1 Regressions

We perform nonlinear regression on the data by finding the polynomial model that maximizes the Bayesian posterior model evidence. We do this in three steps, following the approach outlined in ref. [1]. First, we assume a class of probabilistic models for the data. For each model from the class, we then find the model parameters that maximize the posterior probability, given the model. Finally, we use these model regressions to evaluate which model has the highest posterior probability. In practice, this procedure depends on the choice of model parameterization and the choice of prior for the models and the parameters. We use two separate classes of probabilistic generative models when performing these regressions, one for regressing continuous data and one for regressing discrete data.

For continuous data, we use the following class of probabilistic models for the data. First, we normalize both the dependent and regressor variables by their mean and standard deviation, such that they are mean 0 and variance 1. Next, we model the dependent variable as a function of the regressor variables, plus additive i.i.d. Gaussian noise of mean 0 and variance $\sigma^2$: $y_i = f(x_{ij}; \theta_\alpha) + \epsilon_i$, where $\theta_\alpha$ are the parameters of the model. We fit both the model parameters and the noise standard deviation $\sigma$. We place a log-normal prior on the noise standard deviation, with mean parameter 0 and variance parameter 1. For $x$ univariate, we choose Chebyshev polynomial series as the class of models. For $x$ multivariate, we take $f(x_{ij}) = \sum_j C_j(x_j)$, where $C_j$ is a Chebyshev series in each of the dependent variables. For both cases, we place priors on the coefficients as normal distributions with mean 0 and variance 1. As Chebyshev polynomials take values between 0 and 1 when the dependent variable is between 0 and 1, this model with this set of priors corresponds to assuming that $y(x)$ varies by roughly one standard deviation when $x$ varies by roughly one standard deviation, with the stochastic and deterministic variation in the data being comparable to one another. Combined, the posterior probability of the model parameters given the model and the data is

$$\begin{aligned}\rho(\theta_\alpha, \sigma | y, \boldsymbol{x}; m) \propto & \prod_i \frac{1}{\sqrt{2\pi\sigma^2}} \times \exp\left(-\frac{1}{2}\left(\frac{y_i - f(x_{ij}, \theta_\alpha)}{\sigma}\right)^2\right) \times \\ & \prod_\alpha \frac{1}{\sqrt{2\pi}} \exp\left(-\frac{\theta_\alpha^2}{2}\right) \times \\ & \frac{1}{\sqrt{2\pi}} \exp\left(-\frac{(\ln\sigma)^2}{2}\right)\end{aligned} \tag{1}$$

where $m$ indexes the model, $x_{ij}, y_i$ are the regressor and dependent variables for each datum, and $f$ is a sum of Chebyshev series in each separate, normalized variable with coefficients $\theta_\alpha$. The first term corresponds to the likelihood, the second the priors on the model parameters, and the third the prior on the noise standard deviation. Including the terms $1/\sqrt{2\pi\sigma^2}$ in the likelihood ensures that the noise level fits to the correct value; the prior on the noise level has little effect on the model fitting.

For regressing discrete data, such as the missingness of a variable or the probability of a fetal heartbeat after transfer, we take a similar approach, but model the probability of success as a Bernoulli trial. We take the probability logit to be the same class of functions as before, *i.e.* the probability per trial is $p = 1/(1 + \exp(-f(x_{ij}, \theta_\alpha)))$ where $f$ is a sum of Chebyshev series in each separate normalized variable.

Given a model from this class of models, we then fit the model's parameters from the posterior, by taking the model's maximum *a posteriori* parameters as point estimates and approximating the errors using a Laplace approximation on the posterior.

After the models have been fit, we perform model selection as outlined in ref [1]. We use a Laplace approximation to evaluate the probability of each model as

$$\rho(m|y, \boldsymbol{x}) = \rho(y|\boldsymbol{x}, \theta^*_\alpha, m) \times \rho(\theta^*_\alpha|m) \times \det(\mathbf{A}/2\pi)^{-1/2} \tag{2}$$

where $\rho(y|\boldsymbol{x}, \theta^*_\alpha, m)$ is the likelihood, $\rho(\theta^*_\alpha|m)$ is the prior distribution, $\theta^*_\alpha$ are the maximum *a posteriori* parameters, and $\mathbf{A} = -\nabla\nabla\rho(\theta_\alpha|y, x; m)$ is the inverse of the parameters' covariance matrix. This procedure is related to the Bayesian Information Criterion [3]; the Bayes Information Criterion is an asymptotic approximation of this procedure in the limit of infinite samples. Qualitatively, the model selection combines two contrasting pieces of information: how well the model fits the data, and how fine-tuned the model's parameters need to be to describe the data. More complex models will in general fit the data better (*i.e.* have a higher likelihood), but will in general need more fine-tuning of their parameters (*i.e.* have a smaller determinant of the covariance matrix).

Since there are an infinite number of models in the space of models that we have assumed, we cannot fit all possible models and choose the one with the highest posterior probability. Instead, we search for the most probable

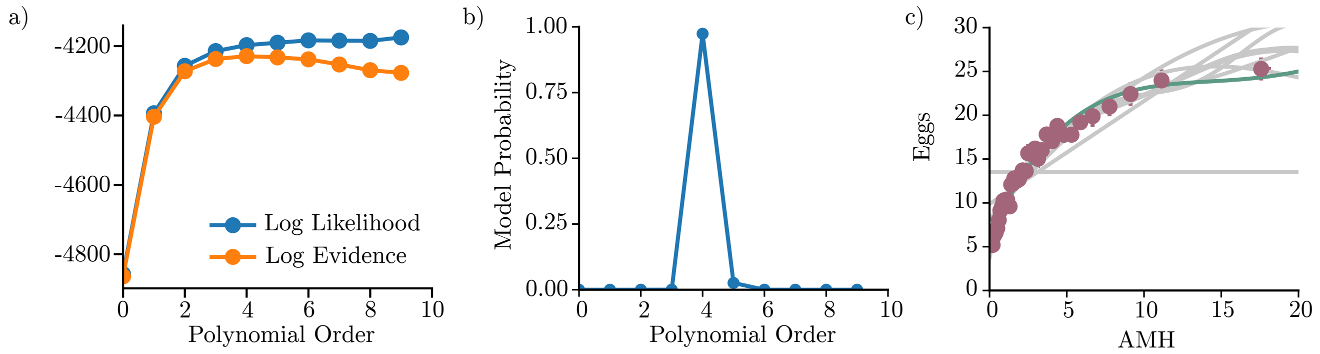


Figure 1: (a) The log-likelihood (blue) and log-evidence (orange) for polynomial models of degree 0-9, for regressing Eggs vs AMH. (b) The corresponding model probabilities. (c) The resulting regressions. Green line: maximum a-posteriori model, corresponding to a fourth-order polynomial. Gray lines: regressions corresponding to the models of other order. Red dots and error bars: mean ± standard error of Eggs vs AMH, after binning into 40 bins with equal counts per bin. The maximum a-posteriori model captures the nonlinearities in the data without overfitting. Compare to SI Fig. 4, which shows the maximum a-posteriori regression with the raw data for Eggs vs AMH.

model as follows. For univariate models, we exhaustively check all polynomial orders up to 8–10 and select the best model found, which is always less than the highest polynomial order checked. For multivariate models, we use the following heuristic search. Each point in the model space can be represented by a tuple of integers, with each integer representing the polynomial degree for the corresponding independent variable. To find the most probable model, we start by fitting the data to a quadratic in each variable. We then iteratively proceed by taking the best model found so far, increasing or decreasing one of the polynomial degrees individually, and re-fitting the model. If neither increasing nor decreasing any of the polynomial orders results in a better fit model, the algorithm terminates the search. For instance, when fitting MII to both Eggs and E2, the algorithm starts by fitting a second-order polynomial in both MII and E2, which can be represented by the point (2, 2).

The algorithm then checks the models (1, 2), corresponding to a model which is linear in Eggs and quadratic in E2, and finds that it is more probable than (2, 2). Next, the algorithm checks the point (0, 2). This is not more probable than (1, 2), so the algorithm proceeds to check the point (1, 1), which is linear in both Eggs and E2. This model is the most favored. The algorithm then checks the points (0, 1) and (1, 0), and finds that they are not favored over (1, 1). At this time, every point adjacent to the best point found so far has been checked, so the algorithm terminates, returning (1, 1) as the most likely model.

In practice, this process results in excellent fits to the data with well-defined model orders. We illustrate this with the regression of Eggs on AMH, shown in Fig. 1. Panel a shows the model probability and model likelihood as a function of the polynomial degree. The model likelihood continues to increase as the polynomial degree increases. In contrast, the model log-evidence attains a maximum at a fourth-degree polynomial; models with higher polynomial degrees require an unfavorable fine-tuning of parameters. Transforming these log-evidences to model probabilities gives a single model that is strongly preferred, with a probability of 97.4%, as shown in panel b. This model visually fits the data best, as illustrated by panel c. This process also performs accurately on generated data. For data generated with a linear model, this formalism identifies a linear model as the one that best fits the data. Likewise, for data generated with a quadratic model, the formalism identifies a quadratic model as best fitting the data. We implement these two as unit tests for our regression framework.

Likewise, for data generated with a linear model, for example,

The results of the analyses in the main text are broadly robust to conditioning via this nonlinear regression vs a linear regression, although we do see some differences. One noticeable difference is in the graph in Fig. 3 in the main text. When we regress Eggs nonlinearly on AMH and HMG, we find that FSH is uncorrelated with Eggs, corresponding to a physiological regime where roughly all possible follicles are recruited by FSH. In contrast, conditioning using linear regression only gives a conditional correlation of FSH and Eggs that is statistically significantly negative, corresponding to a physiological regime where increasing FSH results in fewer recruited follicles. This apparent negative correlation arises because the mean of Eggs is increasing but concave-down as a function of AMH, whereas the mean of FSH is decreasing but concave-up as a function of AMH. As a result, linearly regressing on AMH overestimates Eggs and underestimates FSH when AMH is low. Since the distribution of AMH is skewed, taking the correlation coefficient of these biased residuals then gives a negative correlation.

## 1.2 Estimating Fetal Heartbeat Probabilities

To estimate the probability of an embryo implanting, we use a forward (or generative) model and a Bayesian approach. We assume some class of models, each of which provides a probability of each embryo to develop sufficiently to provide a fetal heartbeat. We then use Bayes theorem to re-cast the probability distribution of fetal heartbeats, given both the model parameters and the number of embryos transferred, into a posterior distribution of the parameters given the measured number of fetal heartbeats and known number of embryos transferred, following the same approach outlined for the continuous regression. Here, we explain in the forward model for fetal heartbeats in more detail.

In each cycle, $n$ embryos are transferred that result in $h$ measured fetal heartbeats. We assume that each embryo has a probability $p_e$ of leading to one fetal heartbeat, and a probability $1 - p_e$ of providing no fetal heartbeat, where the subscript $e$ denotes the which embryo. For simplicity, we ignore the possibility of a single embryo forming monozygotic twins, which demographic data suggests should be a 1% correction. For the few cycles that do have more fetal heartbeats recorded than embryos transferred, we treat every embryo as successfully implanting. Then the probability $p(h|n, \{p_e\})$ is given by a Poisson-binomial distribution. For instance, if two embryos were transferred and one heartbeat was observed, then

$$p(h = 1|n = 2, \{p_e\}) = p_1(1 - p_2) + (1 - p_1)p_2 \quad , \tag{3}$$

where the subscript $e$ indexes embryos and the subscript $c$ indexes cycles.

The data is a collection of many treatment cycles, each with $n_c$ embryos transferred and $h_c$ fetal heartbeats measured. We treat each cycle as an independent event, and therefore the probability of the observed data is

$$p(\{h_c\}|\{n_c\}, \{p_{ec}\}) = \prod_c p(h_c|n_c, \{p_e\}_c) \tag{4}$$

where each $p(h_c|n_c, \{p_e\}_c)$ is a Poisson-binomial distribution.

To proceed further, we assume a functional form for the implantation probabilities $p_{ec}$. Each embryo has some associated parameters $\boldsymbol{x}_{ec}$ with it, such as the number of cells on day 3, the stage on day 5, the age of the woman, *etc.* We assume that the probability of forming a heartbeat depends on the parameters with some functional form $f$, which we parameterize with some set of parameters $\theta_\alpha$: $p_{ec} = p(\boldsymbol{x}_{ec}, \theta_\alpha)$. Substituting this into equation 4 allows writing of the probability of the forward model in terms of the (unknown) model parameters $\theta_\alpha$ and the (known) embryo parameters $\boldsymbol{x}_{ec}$:

$$p(\{h_c\}|\{n_c\}, \theta_\alpha, \{\boldsymbol{x}_{ec}\}) = \prod_c p(h_c|n_c, \{p(\boldsymbol{x}_e; \theta_\alpha)\}_c) \tag{5}$$

We then fit the data with two types of models: smooth, low-dimensional models containing a few number of parameters, and with "model-independent" models that do not assume underlying smoothness of the functional form of $p(\boldsymbol{x}_{ec})$. For the low-dimensional models, we use the same approach as described earlier, parameterizing the logits with a Chebyshev series in the normalized input variables. For the model-independent approaches, we define $p(\boldsymbol{x}; \theta_\alpha)$ as a piecewise-constant function over a series of intervals, by setting the parameters $\theta_\alpha$ to the probability logits on each interval. For example, to calculate a model-independent measure of the probability of an embryo implanting given its day-5 stage, we assign one probability of implanting to all stage-1 embryos, another probability for stage-2 embryos, *etc.* For model-independent measures of the effect of age and BMI on embryo implantation potential, we bin the variables into separate intervals and assign the same probability to each interval; we choose the intervals to contain the same number of embryos (so the intervals are not of equal width). We place a prior on the logits that corresponds to a flat prior of the probabilities ($\rho(\ell) = \text{sech}^2(\ell/2)/4$, where $\ell$ is the logit). While this prior on the logit corresponds to a uniform prior for the fitted probability, this prior does have a maximum and therefore shifts the posterior maximum slightly from the maximum likelihood value. The low dimensional models should balance out variance and bias tradeoff; the model-independent models should be higher variance but do not make any assumptions about smoothness and therefore should have lower bias. These two models are plotted as the green lines and red dots, respectively, in Fig. 5 in the main text and in Fig. 6 in the SI.

After fitting the models, we perform Bayesian model selection, following the same formalism as described above for the regression models. To perform this model selection on day-3 vs day-5 variables, we only use the cycles that have data recorded for both day-3 and day-5. In principle the day-3-only cycles contain information about model selection, but to avoid subtleties due to other confounders we ignore these when performing model selection. In addition, we also limit the data to cycles with 4 or fewer embryo transfers (roughly 90% of the cycles with transfers), to avoid possible confounders when many embryos are transferred.

This approach for estimating the probability of fetal heartbeat assumes that embryos implant independently of one another in multiple transfers. We check this assumption by performing additional regressions with the number of

transferred embryos as a variable. The regression results are consistent with multiple transfers systematically neither helping nor hurting the chance of an individual embryo to implant, as shown in SI Fig. 6g-h. While embryos that are part of a multiple transfer are much less likely to implant than those in a single transfer (panel g), this relationship disappears after controlling for the patient's age and the embryo's stage on day 5 (panel h).

## 1.3 Constructing DAGs

To construct the directed acyclic graph, we tailor our approach using prior knowledge of the data, rather than using more general algorithms that are agnostic to prior knowledge. One such agnostic algorithm for constructing directed acyclic graphs is the inductive-causation (IC) algorithm. The IC algorithm proceeds in three steps. In the first step, one draws a fully connected, undirected graph, then removes any edges A—B if there is any set of variables C such that A and B are conditionally independent given C. Once the undirected graph is constructed, then edges are oriented based on the presence of colliders [2]. This algorithm is guaranteed to produce a directed acyclic graph consistent with the data. We find that an IC algorithm does not perform well on the our dataset. The naive application of an IC algorithm constructs graphs that are physiologically nonsensical, presumably due to the finite statistical power we have in identifying whether two variables are conditionally independent. As an illustration from the data, consider the three variables Age, BMI, and E2. As discussed in the text, Age and BMI are weakly correlated, $\mathrm{Corr}(\mathrm{Age}, \mathrm{BMI}) = 0.07$, and BMI and E2 are weakly negatively correlated, $\mathrm{Corr}(\mathrm{BMI}, \mathrm{E2}) = -0.11$. However, Age and E2 appear uncorrelated, given nothing: $\mathrm{Corr}(\mathrm{Age}, \mathrm{E2}) = -0.02$ ($P = 0.34$). An IC algorithm would suggest drawing the graph with the edges Age $\rightarrow$ BMI and E2 $\rightarrow$ BMI, suggesting that the patient's maximum estradiol concentration recorded during an IVF treatment is what determines whether or not she is overweight. This is especially absurd as some patients have multiple treatment cycles with different recorded E2 but the same BMI. Presumably, the apparent conditional independence between Age and E2 would disappear if much more data was collected. To avoid these types of difficulties, we enforce some prior knowledge in the structure of the directed acyclic graph, although we keep the prior knowledge to the minimum to minimize confirmation bias. Similar problems apply to using a LASSO approach to construcing the directed acyclic graphs.

## 2 Data description

The clinicians score embryos on day 3 and day 5 according to the following procedures:

- **Day 3 Cells**: The number of cells on day 3.
- **Day 3 Fragmentation**: The volume percent of the embryo occupied by fragments, scored as 0%, 1–10%, 11–25%, 26–50%, and >50%.
- **Day 3 Multinucleation**: Scored as 1 (at least 1 blastomere has more than 1 nucleus) or 0 (otherwise).
- **Day 3 Symmetry**: Scored as 1 (perfect symmetry), 2 (moderately asymmetric), or 3 (severely asymmetric).
- **Day 3 Vacuoles**: Scored as 0 (no vacuoles) or 1 (has vacuoles).
- **Day 3 Granularity**: Scored as 0 (not granular) or 1 (granular).
- **Day 5 Stage**: Scored from 1–9, as
  1. Degenerate or arrested; the embryo failed to develop to the morula stage.
  2. Morula, with incomplete compaction (less than 50% compacted).
  3. Morula, with more than 50% of the embryo compacted, but no blastocyst formation visible.
  4. Early blastocyst, where the blastocoele is less than half the volume of the embryo, with little to no expansion in the embryo's volume. The zona pellucida has not started thinning.
  5. Expanding Blastocyst, where the blastocoele occupies more than half the embryo's volume, with some expansion in the embryo's size and the zona pellucida starting to thin.
  6. Full blastocyst, where the blastocoele completely fills the embryo but the zona pellucida has not completely thinned.
  7. Expanded Blastocyst, where the blastocoele completely fills the embryo, which has fully expanded. The zona pellucida is very thin.
  8. Hatching Blastocyst, where the trophectoderm is starting to herniate through the zona pellucida.
  9. Hatched Blastocyst, where the blastocyst is completely hatched out of the zona pellucida.
- **Day 5 ICM**: Scored as a grade from 1–4, with
  1. ICM (inner cell mass) prominent and easily discernible, with many cells that are compacted and tightly adhered together.
  2. ICM discernible, but with fewer cells, and loosely adherent together.
  3. Very few cells visible, either compacted or loose. ICM cells be difficult to distinguish from trophectoderm.
  4. No cells visible in the ICM, or all cells are degenerate or necrotic.

  This is only scored for blastocysts (*i.e.* stage 5 and above).
- **Day 5 Trophectoderm**: Scored as a grade from 1–4, with
  1. A continuous layer of small, uniform, eye-shaped cells bordering the blastocoele.
  2. Fewer, larger cells that may not form a continuous layer.
  3. Sparse trophectoderm cells, which may be large.
  4. All trophectoderm cells are degenerate.

  This is only scored for blastocysts (*i.e.* stage 5 and above).

# 3 Structural Equations corresponding to Models

## 3.1 Structural models for Ovarian Stimulation and Pre-implantation Development

As explained in Sec. 1.1, we assume that the data is normally distributed, with a constant standard deviation and a mean that depends on the dependent variables. In reality, the data show strong evidences of heteroskedasticity and non-normality, cf. Fig. 3 in the main text. Nevertheless these structural models give a reasonably accurate description of the data.

The structural models for ovarian stimulation are calculated using a complete-case basis, since the missingness patterns appears to be correlated with changing clinical practices over time and not with any of the variables. There are 3422 cycles in the train set which have all of AMH, Eggs, MII, and E2 recorded, but 9 of these cycles are missing at least one of Age, BMI, FSH, or HMG. These missing 9 cycles are responsible for the small difference in the MII structural equations between that for the 4-element model and the 8-element model. Differences between other equations correspond to the effects of including other variables.

The structural models for pre-implantation development are calculated using all the data available for each equation; as such, different embryos and cycles are used to model the effect of Age on Day 3 Cells than are used to model Age on Day 5 Stage. In all these equations, Age is measured in years, BMI in kg / $m^2$, E2 is measured in pg / mL, and AMH is measured in international units (IU). The equations for FSH and HMG describe dosage in ampules; one ampule of FSH contains 150 IU, whereas one ampule of HMG contains 75 IU each of LH and FSH. The Day 3 and Day 5 variables are measured as described in Sec. 2.

### 3.1.1 Structural models for Ovarian Stimulation, Main Text Fig. 1

$$\begin{aligned} \text{AMH} =& N(\mu, \sigma^2), \text{with} \\ \mu =& 3.100 \\ \sigma =& 3.706 \end{aligned} \tag{6}$$

$$\begin{aligned} \text{Eggs} =& N(\mu, \sigma^2), \text{with} \\ \mu =& 6.078 + \\ & 3.938 \times \text{AMH} - 0.325 \times \text{AMH}^2 + 0.012 \times \text{AMH}^3 - 1.38 \times 10^{-4} \times \text{AMH}^4 \\ \sigma =& 7.359 \end{aligned} \tag{7}$$

$$\begin{aligned} \text{E2} =& N(\mu, \sigma^2), \text{with} \\ \mu =& 9.76 \times 10^2 + \\ & 96.252 \times \text{Eggs} - 0.957 \times \text{Eggs}^2 \\ \sigma =& 8.89 \times 10^2 \end{aligned} \tag{8}$$

$$\begin{aligned} \text{MII} =& N(\mu, \sigma^2), \text{with} \\ \mu =& 0.133 + \\ & 0.695 \times \text{Eggs} + \\ & 2.66 \times 10^{-4} \times \text{E2} \\ \sigma =& 2.929 \end{aligned} \tag{9}$$

### 3.1.2 Structural models for Ovarian Stimulation, Main Text Fig. 3

$$\begin{aligned} \text{Age} =& N(\mu, \sigma^2), \text{with} \\ \mu =& 36.563 \\ \sigma =& 4.357 \end{aligned} \tag{10}$$

$$\begin{aligned}\text{BMI} =& N(\mu,\sigma^2), \text{with}\\ \mu =& 22.087+\\ & 0.110 \times \text{Age}\\ \sigma =& 6.570\end{aligned} \tag{11}$$

$$\begin{aligned}\text{AMH} =& N(\mu,\sigma^2), \text{with}\\ \mu =& 12.066+\\ & -0.245 \times \text{Age}\\ \sigma =& 3.543\end{aligned} \tag{12}$$

$$\begin{aligned}\text{FSH} =& N(\mu,\sigma^2), \text{with}\\ \mu =& 11.669+\\ & 0.653 \times \text{Age}+\\ & 0.172 \times \text{BMI}+\\ & -7.928 \times \text{AMH} + 0.780 \times \text{AMH}^2 - 0.029 \times \text{AMH}^3 + 3.49 \times 10^{-4} \times \text{AMH}^4\\ \sigma =& 15.516\end{aligned} \tag{13}$$

$$\begin{aligned}\text{HMG} =& N(\mu,\sigma^2), \text{with}\\ \mu =& 56.312+\\ & -2.893 \times \text{Age} + 0.054 \times \text{Age}^2+\\ & -20.019 \times \text{AMH} + 4.181 \times \text{AMH}^2 - 0.389 \times \text{AMH}^3 + 0.018 \times \text{AMH}^4+\\ & -3.73 \times 10^{-4} \times \text{AMH}^5 + 2.99 \times 10^{-6} \times \text{AMH}^6+\\ & 0.627 \times \text{FSH} - 5.73 \times 10^{-3} \times \text{FSH}^2\\ \sigma =& 14.878\end{aligned} \tag{14}$$

$$\begin{aligned}\text{Eggs} =& N(\mu,\sigma^2), \text{with}\\ \mu =& 8.039+\\ & 2.451 \times \text{AMH} - 0.114 \times \text{AMH}^2 + 1.59 \times 10^{-3} \times \text{AMH}^3+\\ & -0.066 \times \text{HMG}\\ \sigma =& 7.308\end{aligned} \tag{15}$$

$$\begin{aligned}\text{E2} =& N(\mu,\sigma^2), \text{with}\\ \mu =& 1.14 \times 10^3+\\ & 26.308 \times \text{Age}+\\ & -14.213 \times \text{BMI}+\\ & -4.655 \times \text{FSH}+\\ & 13.637 \times \text{HMG} - 0.169 \times \text{HMG}^2+\\ & 1.04 \times 10^2 \times \text{Eggs} - 1.042 \times \text{Eggs}^2\\ \sigma =& 8.65 \times 10^2\end{aligned} \tag{16}$$

$$\begin{aligned}\text{MII} =& N(\mu,\sigma^2), \text{with}\\ \mu =& 0.132+\\ & 0.695 \times \text{Eggs}+\\ & 2.64 \times 10^{-4} \times \text{E2}\\ \sigma =& 2.932\end{aligned} \tag{17}$$

### 3.1.3 Structural models for Pre-Implantation Development, Main Tex Fig. 5

$$\begin{aligned}\text{BMI} =& N(\mu, \sigma^2), \text{with} \\ \mu =& 21.557+ \\ & 0.123 \times \text{Age} \\ \sigma =& 6.428\end{aligned} \tag{18}$$

$$\begin{aligned}\text{MII} =& N(\mu, \sigma^2), \text{with} \\ \mu =& 42.519+ \\ & -1.494 \times \text{Age} + 0.016 \times \text{Age}^2 \\ \sigma =& 6.571\end{aligned} \tag{19}$$

$$\begin{aligned}\text{Day 3 Cells} =& N(\mu, \sigma^2), \text{with} \\ \mu =& 8.783+ \\ & -0.038 \times \text{Age} \\ \sigma =& 2.429\end{aligned} \tag{20}$$

$$\begin{aligned}\text{Day 5 Stage} =& N(\mu, \sigma^2), \text{with} \\ \mu =& 3.642+ \\ & 0.063 \times \text{Age} - 1.58 \times 10^{-3} \times \text{Age}^2 + \\ & 0.847 \times \text{Day 3 Cells} - 0.031 \times \text{Day 3 Cells}^2 \\ \sigma =& 1.828\end{aligned} \tag{21}$$

$$\begin{aligned}P(\text{Fetal Heartbeat}) =& (1 + e^{-z})^{-1}, \text{with} \\ z =& -8.704+ \\ & 0.543 \times \text{Age} - 9.18 \times 10^{-3} \times \text{Age}^2 + \\ & 0.292 \times \text{Day 5 Stage}\end{aligned} \tag{22}$$

We present the missingness structural equations here for completeness. Empirically, the distribution of whether an embryo is transferred (*i.e.* missingness for fetal heartbeat) differs for embryos transferred on day 3 versus those on day 5; we present both here as separate equations.

$$\begin{aligned}P(\text{D5 Rec.}) =& (1 + e^{-z})^{-1}, \text{with} \\ z =& -3.588+ \\ & 0.923 \times \text{MII} - 0.054 \times \text{MII}^2 + 1.35 \times 10^{-3} \times \text{MII}^3 - 1.12 \times 10^{-5} \times \text{MII}^4 + \\ & -2.587 \times \text{Age} + 0.089 \times \text{Age}^2 - 9.95 \times 10^{-4} \times \text{Age}^3 + \\ & 4.369 \times \text{Day 3 Cells} - 1.222 \times \text{Day 3 Cells}^2 + 0.147 \times \text{Day 3 Cells}^3 - \\ & 7.91 \times 10^{-3} \times \text{Day 3 Cells}^4 + 1.57 \times 10^{-4} \times \text{Day 3 Cells}^5 + \\ & -0.129 \times \text{BMI} + 1.99 \times 10^{-3} \times \text{BMI}^2\end{aligned} \tag{23}$$

$$\begin{aligned}P(\text{Trans.}|\text{D5 Rec.}) =& (1 + e^{-z})^{-1}, \text{with} \\ z =& -3.776+ \\ & 0.129 \times \text{MII} - 9.82 \times 10^{-3} \times \text{MII}^2 + 1.23 \times 10^{-4} \times \text{MII}^3 + \\ & 1.604 \times \text{Age} - 0.056 \times \text{Age}^2 + 6.42 \times 10^{-4} \times \text{Age}^3 + \\ & 2.300 \times \text{Day 3 Cells} - 0.223 \times \text{Day 3 Cells}^2 + 6.60 \times 10^{-3} \times \text{Day 3 Cells}^3 + \\ & 1.090 \times \text{Day 5 Stage} - 0.029 \times \text{Day 5 Stage}^2\end{aligned} \tag{24}$$

$$
\begin{aligned}
P(\text{Trans.}|\text{D5 Miss.}) =& (1+e^{-z})^{-1}, \text{with} \\
z =& 6.151+ \\
& -0.760 \times \text{MII} + 0.028 \times \text{MII}^2 - 2.92 \times 10^{-4} \times \text{MII}^3 + \\
& 1.977 \times \text{Age} - 0.076 \times \text{Age}^2 + 9.52 \times 10^{-4} \times \text{Age}^3 + \\
& 1.568 \times \text{Day 3 Cells} - 0.082 \times \text{Day 3 Cells}^2
\end{aligned} \tag{25}
$$

# 4 Supporting Data & Graphs for claims in the main text

## 4.1 Cross-Validation Results

The rank plot in Figure 3b in the main text shows the measured P-values for 99 conditional correlations among the 8 variables corresponding to the 99 conditional independencies predicted by the model in Figure 3a in the main text. To create this plot, we measure the conditional correlation and associated P-value (without a Bonferroni correction) for each conditional correlation in both the train and test sets. The table at the end of this section shows all measured P-values on the test and train sets; note that the conditional correlations with suspiciously low P-values on the test set typically do not have low P-values on the train set, and vice versa.

To generate the rank plots simulated according to the proposed model (Main Text Figure 3b), we start by generating 3,000 datasets according to the model in Figure 3a. To do so, we first randomly sample Age with replacement. We then generate the BMI by combining the structural equations from Main Text Figure 3a and SI Section 3 with the randomly-sampled (with replacement) residuals from the fit of BMI to the train data. We then continue this process by proceeding down the graph in Main Text Figure 3a to calculate AMH, then FSH, HMG, *etc.* For each simulated dataset, we then calculate the 99 conditional correlations by performing the necessary regressions with the same polynomial degree used for the real data and calculating the correlation between the residuals. These simulated P-value rank plots give an estimate of what would be expected if the model proposed in the main text is true. In principle, the distribution of P-value ranks for those generated according to the train data procedure, where each dataset containg 3,413 cycles and the conditional correlations are evaluated by regressing on that dataset, differs from the rank distribution generated according to the test data procedure, where each dataset contains 1,497 cycles and the conditional correlations are evaulated using regressions on the train data. In practice, the differences between these distributions are not visible; as such, Main Text Figure 3 just shows the distribution for the simulated train data. For comparison, we also generate rank plots according to linear Gaussian fully-connected models (Main Text Figure 3c). For this, we first generate 3,000 datasets according to a random Gaussian models, each with a randomly-drawn covariance matrix $C = UU^T$, where $U_{ij}$ is a Gaussian random variable with mean 0 and variance 1. We then calculate the 99 conditional correlations for each of those 3,000 datasets, performing the regressions with the same polynomial degree used for the real data and the previously simulated data.

We quantify the similarity between the expected and measured rank plots in Main Text Figure 3b with two statistics. First, we examine the maximum distance between the measured P-value ranks and the median expected from the simulation (*i.e.* the maximum vertical separation between the black line and the red or green lines in the figure), similar to a Kolmogorov-Smirnov test. The maximum distance for the P-values measured on the train set is 0.33; 0.09 of the simulated rank curves have this maximum distance or greater. The maximum distance for the P-values measured on the test set is 0.24; 0.31 of the simulated rank curves have this maximum distance or greater. This first statistic suggests that the proposed model broadly agrees with the data. Second, we examine the minimum P-value for the 99 conditional independencies. The minimum P-value measured on the training set is $2 \times 10^{-4}$ (corresponding to $\mathrm{Corr}(\mathrm{AMH}, \mathrm{E2} \mid \mathrm{Age}, \mathrm{BMI}, \mathrm{FSH}, \mathrm{HMG}, \mathrm{Eggs}, \mathrm{MII})$); only 0.004 of the simulated rank curves have a P-value this low. The minimum P-value measured on the test set is $7 \times 10^{-5}$ (corresponding to $\mathrm{Corr}(\mathrm{Age}, \mathrm{Eggs} \mid \mathrm{AMH}, \mathrm{FSH}, \mathrm{HMG})$); only 0.001 of the simulated rank curves have a P-value this low. Thus, this second statistic weakly suggests that some features are missing from the model. Combined, this analysis shows that the model in Main Text Fig. 3 is broadly consistent with the data, although with some evidence for additional, small physiological effects missing from the model.

We also meaure how much the variance of the residuals changes when including all possible parameters, for both the ovarian stimulation graph and the development graph. To do this, we fit the train data assuming a completely connected graph. We nonlinearly regress each variable on all the upstream variables, following the procedure outlined in Sec. 1.1 but forcing each term to enter in at least linearly. We then measure the variance of the residuals on the test set, and compare the variance to the residuals on the test set using the model proposed in the main text. Of the 8 ovarian stimulation variables shown in Fig. 3 in the main text, 3 remain unchanged on changing to a fully connected model: Age is the first variable in both graphs and has no edges pointing into it, BMI is the second variable in both graphs and therefore only has Age pointing into it, and FSH has all upstream variables pointing into it in the fully connected model. The variance change for the remaining 5 variables is shown in the table below. Using a complete model worsens the fits for all but Eggs. This worsening is presumably due to the increased variance in the regression estimate when including additional variables. For pre-implantation development, the variance of the Day 3 Cells residuals decreases when including MII and BMI, whereas the variance of the Day 5 Stage residuals increases.

| Name | Test Set Var., proposed model | Test Set Var., complete model | Percent change |
|---|---|---|---|
| AMH | 15.18 | 15.20 | +0.153% |
| HMG | 251.27 | 251.45 | +0.071% |
| Eggs | 51.68 | 51.37 | -0.600% |
| E2 | 883,606 | 888,766 | +0.584% |
| MII | 8.98 | 8.99 | +0.182% |
| Day 3 Cells | 5.78 | 5.77 | -0.184% |
| Day 5 Stage | 3.40 | 3.40 | +0.034% |

To check the results for fetal heartbeat, we use a likelihood test. We fit two models on the train set, the model proposed in Main Text Fig. 5 and a complete model that includes additional parameters as described above. We then fix the model parameters to their maximum *a posteriori* values and calculate the likelihood of the models on the test set. Since the models are fit on the train set and evaluated on the test set, the ratio of the likelihood corresponds to a Bayesian odds ratio of the two models; the table below reports this as a probability of the model in the text being correct. The first row compares the model Age, Day 5 Stage → FH against the model Age, BMI, MII, Day 3 Cells, Day 5 Stage → FH; the second row compares the model Age, Day 5 Troph, Day 5 Stage → FH against Age, Day 3 Cells, Day 3 Frag, Day 3 Granularity, Day 3 Multinucleation, Day 3 Symmetry, Day 3 Vacuoles, Day 5 Stage, Day 5 ICM, Day 5 Trophectoderm → FH. The two sets of likelihood are not directly comparable, as not all Day 5 transfers have the trophectoderm and ICM grade recorded (these are only recorded for developed blastocysts of stage 5 or higher).

| Name | Log Likelihood, proposed | Log Likelihood, complete | P |
|---|---|---|---|
| Including BMI, MII, and Day 3 Cells | -479.96 | -478.14 | 0.14 |
| Including all Day 3, Day 5 grades | -415.51 | -415.61 | 0.53 |

| Name | Corr., Train | $P$, Train | Corr., Test | $P$, Test |
|---|---|---|---|---|
| Corr(Age, Eggs \| AMH, FSH, HMG) | -0.040 | 0.020 | -0.102 | $7 \times 10^{-5}$ |
| Corr(Age, Eggs \| AMH, BMI, FSH, HMG) | -0.040 | 0.020 | -0.102 | $7 \times 10^{-5}$ |
| Corr(Age, Eggs \| AMH, BMI, HMG) | -0.045 | 0.009 | -0.090 | $5 \times 10^{-4}$ |
| Corr(Age, Eggs \| AMH, HMG) | -0.045 | 0.009 | -0.090 | $5 \times 10^{-4}$ |
| Corr(Age, MII \| AMH, E2, Eggs) | 0.012 | 0.467 | -0.055 | 0.034 |
| Corr(Age, MII \| AMH, BMI, E2, Eggs) | 0.013 | 0.453 | -0.054 | 0.038 |
| Corr(Age, MII \| AMH, E2, FSH, Eggs) | 0.009 | 0.615 | -0.053 | 0.041 |
| Corr(Age, MII \| AMH, BMI, E2, FSH, Eggs) | 0.009 | 0.615 | -0.053 | 0.041 |
| Corr(Age, MII \| E2, Eggs) | 0.016 | 0.351 | -0.053 | 0.042 |
| Corr(Age, MII \| BMI, E2, Eggs) | 0.016 | 0.338 | -0.051 | 0.047 |
| Corr(Age, MII \| BMI, E2, FSH, Eggs) | 0.010 | 0.544 | -0.051 | 0.049 |
| Corr(Age, MII \| E2, FSH, Eggs) | 0.010 | 0.544 | -0.051 | 0.049 |
| Corr(AMH, MII \| Age, BMI, FSH, HMG, Eggs) | -0.030 | 0.083 | -0.049 | 0.057 |
| Corr(AMH, MII \| Age, E2, FSH, HMG, Eggs) | -0.033 | 0.054 | -0.047 | 0.066 |
| Corr(AMH, MII \| Age, BMI, E2, FSH, HMG, Eggs) | -0.033 | 0.054 | -0.047 | 0.066 |
| Corr(AMH, MII \| BMI, E2, FSH, HMG, Eggs) | -0.035 | 0.043 | -0.047 | 0.071 |
| Corr(AMH, MII \| E2, FSH, HMG, Eggs) | -0.035 | 0.043 | -0.047 | 0.071 |
| Corr(FSH, MII \| E2, HMG, Eggs) | 0.012 | 0.498 | -0.040 | 0.126 |
| Corr(FSH, MII \| BMI, E2, HMG, Eggs) | 0.012 | 0.483 | -0.039 | 0.130 |
| Corr(Age, MII \| AMH, E2, FSH, HMG, Eggs) | 0.029 | 0.093 | -0.039 | 0.131 |
| Corr(Age, MII \| BMI, E2, FSH, HMG, Eggs) | 0.029 | 0.093 | -0.039 | 0.131 |
| Corr(Age, MII \| E2, FSH, HMG, Eggs) | 0.029 | 0.093 | -0.039 | 0.131 |
| Corr(Age, MII \| AMH, BMI, E2, FSH, HMG, Eggs) | 0.029 | 0.093 | -0.039 | 0.131 |
| Corr(HMG, MII \| E2, Eggs) | -0.039 | 0.022 | -0.037 | 0.155 |
| Corr(Age, MII \| AMH, E2, HMG, Eggs) | 0.029 | 0.086 | -0.036 | 0.164 |
| Corr(Age, MII \| AMH, BMI, E2, HMG, Eggs) | 0.029 | 0.085 | -0.036 | 0.169 |
| Corr(HMG, MII \| BMI, E2, Eggs) | -0.039 | 0.022 | -0.035 | 0.175 |
| Corr(FSH, MII \| Age, E2, HMG, Eggs) | 0.003 | 0.874 | -0.034 | 0.183 |
| Corr(FSH, MII \| Age, BMI, E2, HMG, Eggs) | 0.003 | 0.854 | -0.034 | 0.188 |
| Corr(AMH, MII \| Age, BMI, E2, HMG, Eggs) | -0.034 | 0.047 | -0.034 | 0.191 |
| Corr(AMH, MII \| Age, E2, HMG, Eggs) | -0.034 | 0.047 | -0.034 | 0.191 |
| Corr(Age, MII \| E2, HMG, Eggs) | 0.033 | 0.055 | -0.033 | 0.206 |
| Corr(Age, MII \| BMI, E2, HMG, Eggs) | 0.033 | 0.054 | -0.032 | 0.212 |
| Corr(HMG, MII \| AMH, E2, Eggs) | -0.037 | 0.031 | -0.031 | 0.234 |
| Corr(HMG, MII \| AMH, BMI, E2, Eggs) | -0.037 | 0.031 | -0.029 | 0.257 |
| Corr(HMG, MII \| E2, FSH, Eggs) | -0.047 | 0.006 | -0.029 | 0.260 |
| Corr(HMG, MII \| BMI, E2, FSH, Eggs) | -0.047 | 0.006 | -0.028 | 0.272 |
| Corr(FSH, MII \| E2, Eggs) | 0.009 | 0.615 | -0.027 | 0.290 |
| Corr(AMH, MII \| Age, BMI, E2, FSH, Eggs) | -0.017 | 0.328 | -0.027 | 0.296 |
| Corr(AMH, MII \| Age, E2, FSH, Eggs) | -0.017 | 0.328 | -0.027 | 0.296 |
| Corr(BMI, Eggs \| AMH, HMG) | -0.012 | 0.466 | -0.027 | 0.296 |
| Corr(AMH, MII \| Age, BMI, E2, Eggs) | -0.021 | 0.225 | -0.026 | 0.306 |
| Corr(AMH, MII \| Age, E2, Eggs) | -0.021 | 0.225 | -0.026 | 0.306 |
| Corr(HMG, MII \| AMH, E2, FSH, Eggs) | -0.042 | 0.013 | -0.026 | 0.306 |
| Corr(HMG, MII \| AMH, BMI, E2, FSH, Eggs) | -0.042 | 0.013 | -0.026 | 0.322 |
| Corr(FSH, MII \| BMI, E2, Eggs) | 0.009 | 0.586 | -0.025 | 0.325 |
| Corr(AMH, E2 \| Age, BMI, FSH, HMG, Eggs) | 0.061 | $3 \times 10^{-4}$ | -0.024 | 0.355 |
| Corr(BMI, Eggs \| Age, AMH, HMG) | -0.011 | 0.508 | -0.024 | 0.355 |
| Corr(AMH, MII \| BMI, E2, HMG, Eggs) | -0.032 | 0.066 | -0.023 | 0.364 |
| Corr(AMH, MII \| E2, HMG, Eggs) | -0.032 | 0.066 | -0.023 | 0.364 |
| Corr(BMI, Eggs \| AMH, FSH, HMG) | -0.011 | 0.540 | -0.023 | 0.368 |
| Corr(BMI, Eggs \| Age, AMH, FSH) | -0.011 | 0.530 | -0.023 | 0.370 |
| Corr(BMI, Eggs \| Age, AMH, FSH, HMG) | -0.011 | 0.539 | -0.022 | 0.389 |

| Name | Corr., Train | $P$, Train | Corr., Test | $P$, Test |
|---|---|---|---|---|
| Corr(AMH, MII \| BMI, E2, FSH, Eggs) | -0.018 | 0.292 | -0.022 | 0.397 |
| Corr(AMH, MII \| E2, FSH, Eggs) | -0.018 | 0.292 | -0.022 | 0.397 |
| Corr(FSH, MII \| AMH, E2, Eggs) | 0.021 | 0.226 | -0.022 | 0.403 |
| Corr(HMG, MII \| Age, BMI, E2, Eggs) | -0.044 | 0.009 | -0.021 | 0.424 |
| Corr(HMG, MII \| Age, BMI, E2, FSH, Eggs) | -0.049 | 0.004 | -0.021 | 0.425 |
| Corr(HMG, MII \| Age, E2, FSH, Eggs) | -0.049 | 0.004 | -0.021 | 0.425 |
| Corr(AMH, E2 \| Age, BMI, FSH, HMG, Eggs, MII) | 0.064 | $2 \times 10^{-4}$ | -0.020 | 0.429 |
| Corr(FSH, MII \| AMH, BMI, E2, Eggs) | 0.021 | 0.220 | -0.020 | 0.431 |
| Corr(HMG, MII \| Age, E2, Eggs) | -0.042 | 0.014 | -0.018 | 0.475 |
| Corr(BMI, MII \| AMH, E2, Eggs) | -0.005 | 0.785 | -0.018 | 0.487 |
| Corr(BMI, MII \| E2, Eggs) | -0.005 | 0.785 | -0.018 | 0.487 |
| Corr(HMG, MII \| Age, AMH, E2, Eggs) | -0.042 | 0.015 | -0.018 | 0.494 |
| Corr(HMG, MII \| Age, AMH, BMI, E2, FSH, Eggs) | -0.045 | 0.008 | -0.017 | 0.502 |
| Corr(HMG, MII \| Age, AMH, E2, FSH, Eggs) | -0.045 | 0.008 | -0.017 | 0.502 |
| Corr(HMG, MII \| Age, AMH, BMI, E2, Eggs) | -0.042 | 0.015 | -0.017 | 0.515 |
| Corr(BMI, MII \| AMH, E2, FSH, Eggs) | -0.006 | 0.737 | -0.017 | 0.516 |
| Corr(BMI, MII \| E2, FSH, Eggs) | -0.006 | 0.737 | -0.017 | 0.516 |
| Corr(BMI, MII \| AMH, E2, HMG, Eggs) | $-6 \times 10^{-4}$ | 0.971 | -0.016 | 0.535 |
| Corr(BMI, MII \| E2, HMG, Eggs) | $-6 \times 10^{-4}$ | 0.971 | -0.016 | 0.535 |
| Corr(BMI, MII \| E2, FSH, HMG, Eggs) | -0.003 | 0.846 | -0.015 | 0.554 |
| Corr(BMI, MII \| Age, E2, FSH, HMG, Eggs) | -0.003 | 0.846 | -0.015 | 0.554 |
| Corr(BMI, MII \| AMH, E2, FSH, HMG, Eggs) | -0.003 | 0.846 | -0.015 | 0.554 |
| Corr(FSH, Eggs \| AMH, HMG) | -0.040 | 0.019 | -0.015 | 0.571 |
| Corr(BMI, MII \| Age, AMH, E2, Eggs) | -0.005 | 0.751 | -0.014 | 0.577 |
| Corr(BMI, MII \| Age, E2, Eggs) | -0.005 | 0.751 | -0.014 | 0.577 |
| Corr(BMI, MII \| Age, AMH, E2, FSH, HMG, Eggs) | -0.006 | 0.709 | -0.014 | 0.584 |
| Corr(BMI, MII \| Age, AMH, E2, FSH, Eggs) | -0.006 | 0.709 | -0.014 | 0.584 |
| Corr(BMI, MII \| Age, E2, FSH, Eggs) | -0.006 | 0.709 | -0.014 | 0.584 |
| Corr(AMH, MII \| BMI, E2, Eggs) | -0.022 | 0.197 | -0.013 | 0.604 |
| Corr(AMH, MII \| E2, Eggs) | -0.022 | 0.197 | -0.013 | 0.604 |
| Corr(BMI, MII \| Age, AMH, E2, HMG, Eggs) | -0.002 | 0.894 | -0.013 | 0.608 |
| Corr(BMI, MII \| Age, E2, HMG, Eggs) | -0.002 | 0.894 | -0.013 | 0.608 |
| Corr(FSH, MII \| AMH, E2, HMG, Eggs) | 0.008 | 0.655 | -0.013 | 0.619 |
| Corr(FSH, Eggs \| AMH, BMI, HMG) | -0.045 | 0.009 | -0.013 | 0.622 |
| Corr(FSH, MII \| Age, AMH, E2, Eggs) | 0.018 | 0.296 | -0.013 | 0.625 |
| Corr(FSH, MII \| Age, AMH, BMI, E2, Eggs) | 0.018 | 0.288 | -0.012 | 0.650 |
| Corr(FSH, Eggs \| Age, AMH, BMI, HMG) | -0.026 | 0.126 | 0.012 | 0.651 |
| Corr(FSH, Eggs \| Age, AMH, HMG) | -0.027 | 0.119 | 0.012 | 0.654 |
| Corr(FSH, MII \| Age, AMH, E2, HMG, Eggs) | 0.001 | 0.949 | -0.010 | 0.696 |
| Corr(FSH, MII \| AMH, BMI, E2, HMG, Eggs) | 0.004 | 0.821 | -0.010 | 0.698 |
| Corr(FSH, MII \| Age, AMH, BMI, E2, HMG, Eggs) | 0.001 | 0.931 | -0.010 | 0.700 |
| Corr(FSH, MII \| Age, E2, Eggs) | 0.009 | 0.587 | -0.008 | 0.770 |
| Corr(FSH, MII \| Age, BMI, E2, Eggs) | 0.010 | 0.571 | -0.007 | 0.799 |
| Corr(BMI, HMG \| Age, AMH, FSH) | 0.024 | 0.161 | -0.005 | 0.846 |
| Corr(BMI, HMG \| Age, AMH, FSH, Eggs) | 0.025 | 0.137 | -0.003 | 0.913 |
| Corr(AMH, BMI \| Age) | -0.044 | 0.011 | 0.002 | 0.951 |

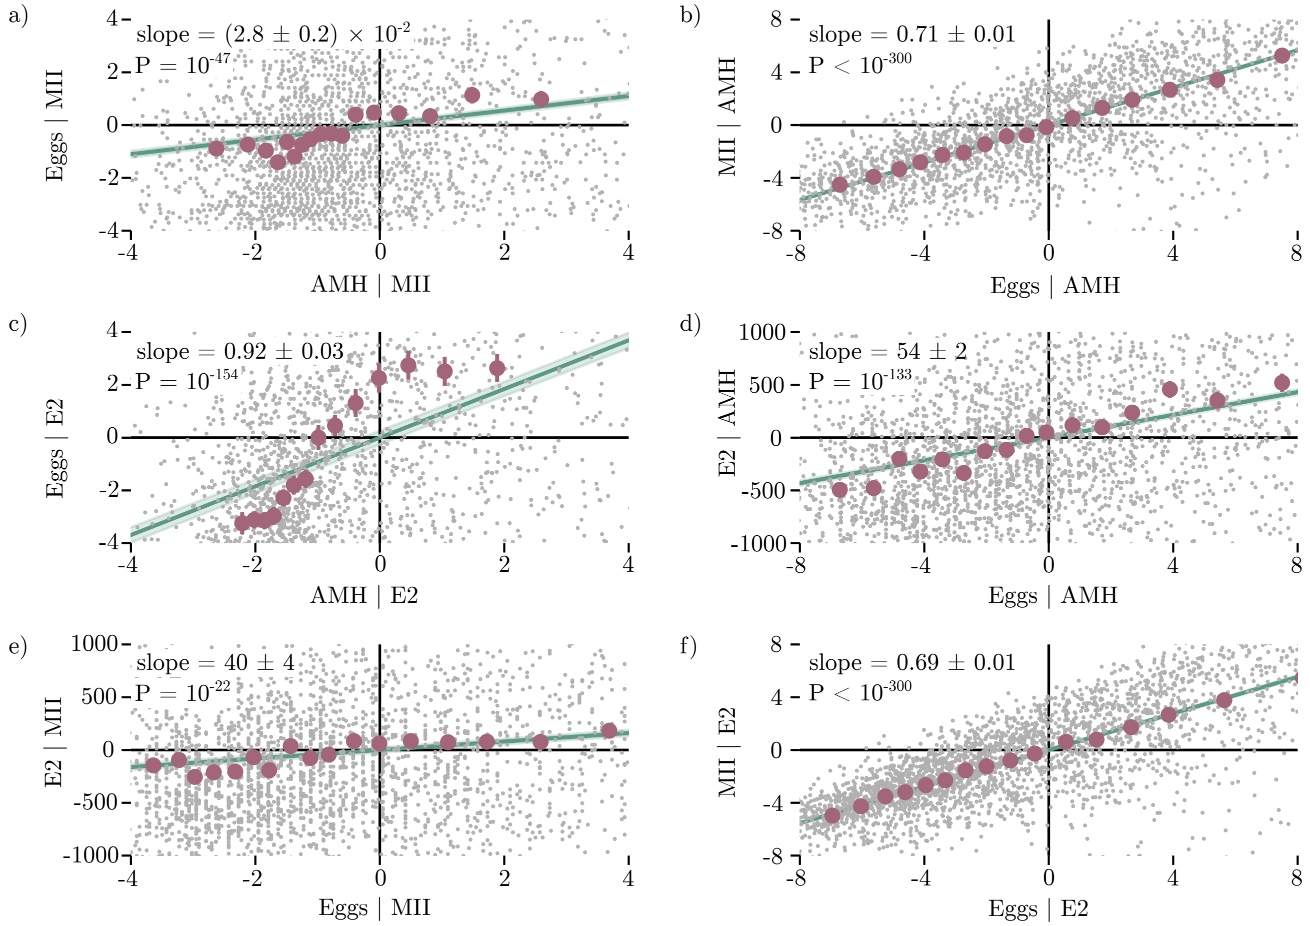


Figure 2: Additional conditional correlations corresponding to Fig. 1 in the main text. The only two conditional independencies apparent in the data are the two shown in Fig. 1 in the main text. (a) The residuals of the Eggs plotted versus the residuals of the patient AMH, after regressing both against MII, which we denote as Eggs vs Age | MII. (b) MII vs Eggs | AMH. (c) Eggs vs AMH | E2. (d) E2 vs Eggs | AMH. (e) E2 vs Eggs | MII. (e) MII vs Eggs | E2.

## 4.2 Oocyte Maturation

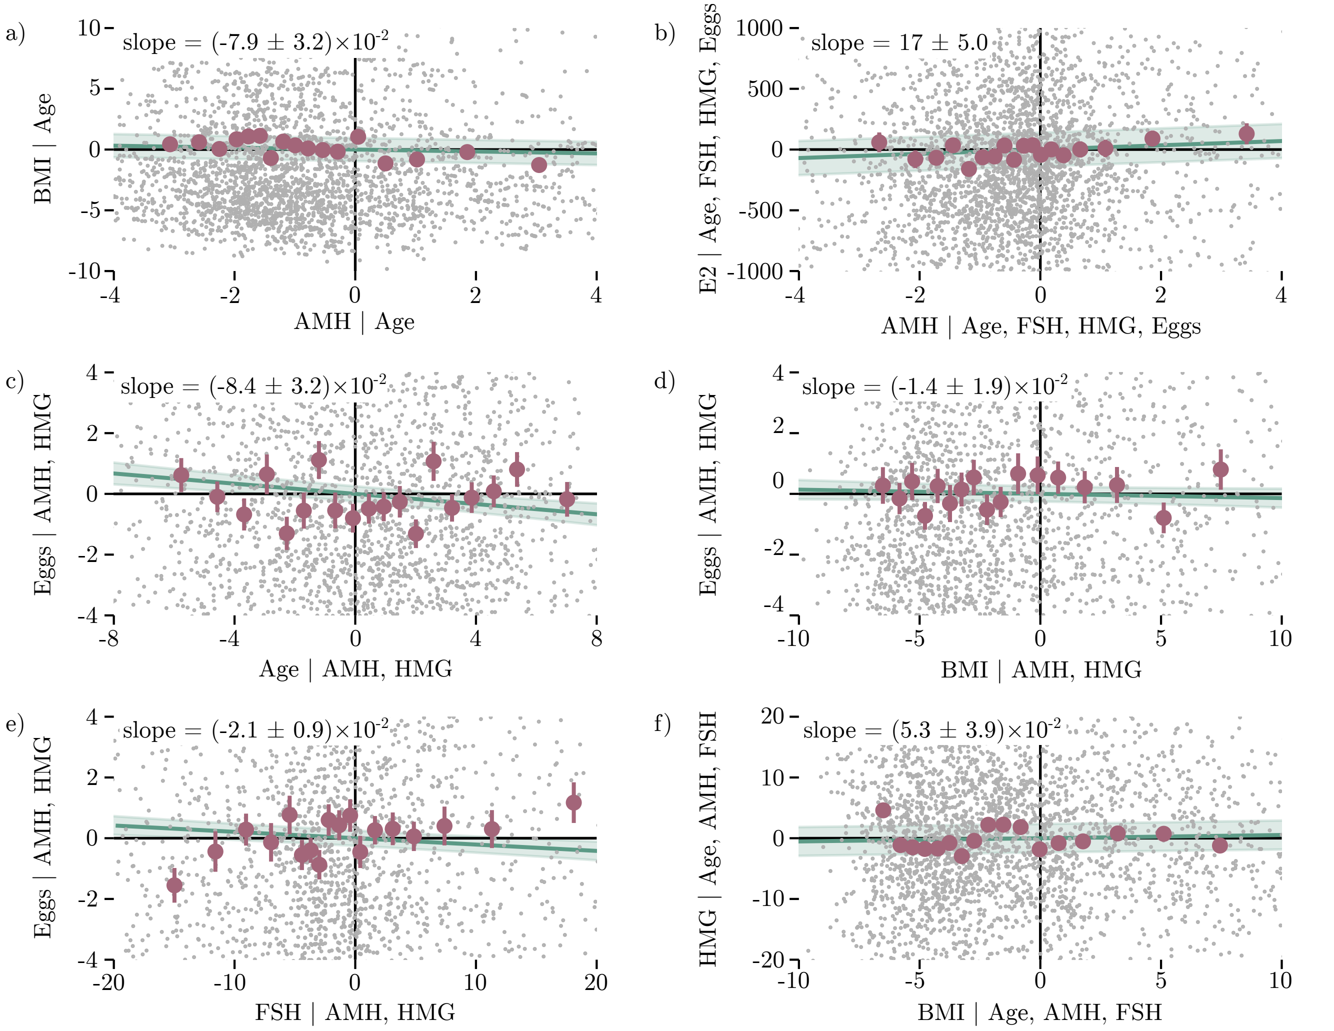


Figure 3: Conditional independencies for the graphical model shown in Fig. 3 in the main text. (a) BMI vs AMH | Age. (b) E2 vs AMH | Eggs, FSH, HMG. (c) Eggs vs AMH | AMH, HMG. (d) Eggs vs BMI | AMH, HMG. (e) Eggs vs FSH | AMH, HMG. (e) HMG vs BMI | Age, AMH, FSH.

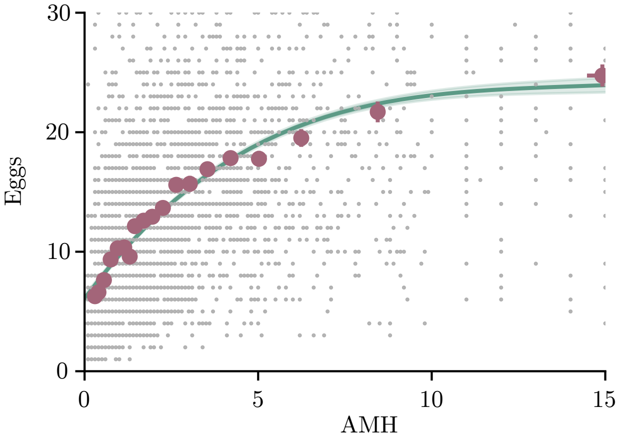


Figure 4: Eggs vs AMH. Green lines: nonlinear fit to the data; red dots: data and standard error after grouping into 20 bins; gray dots: raw data. Note that, while AMH is linear in Eggs (Fig. 3 of main text), AMH is visibly nonlinear in Eggs.

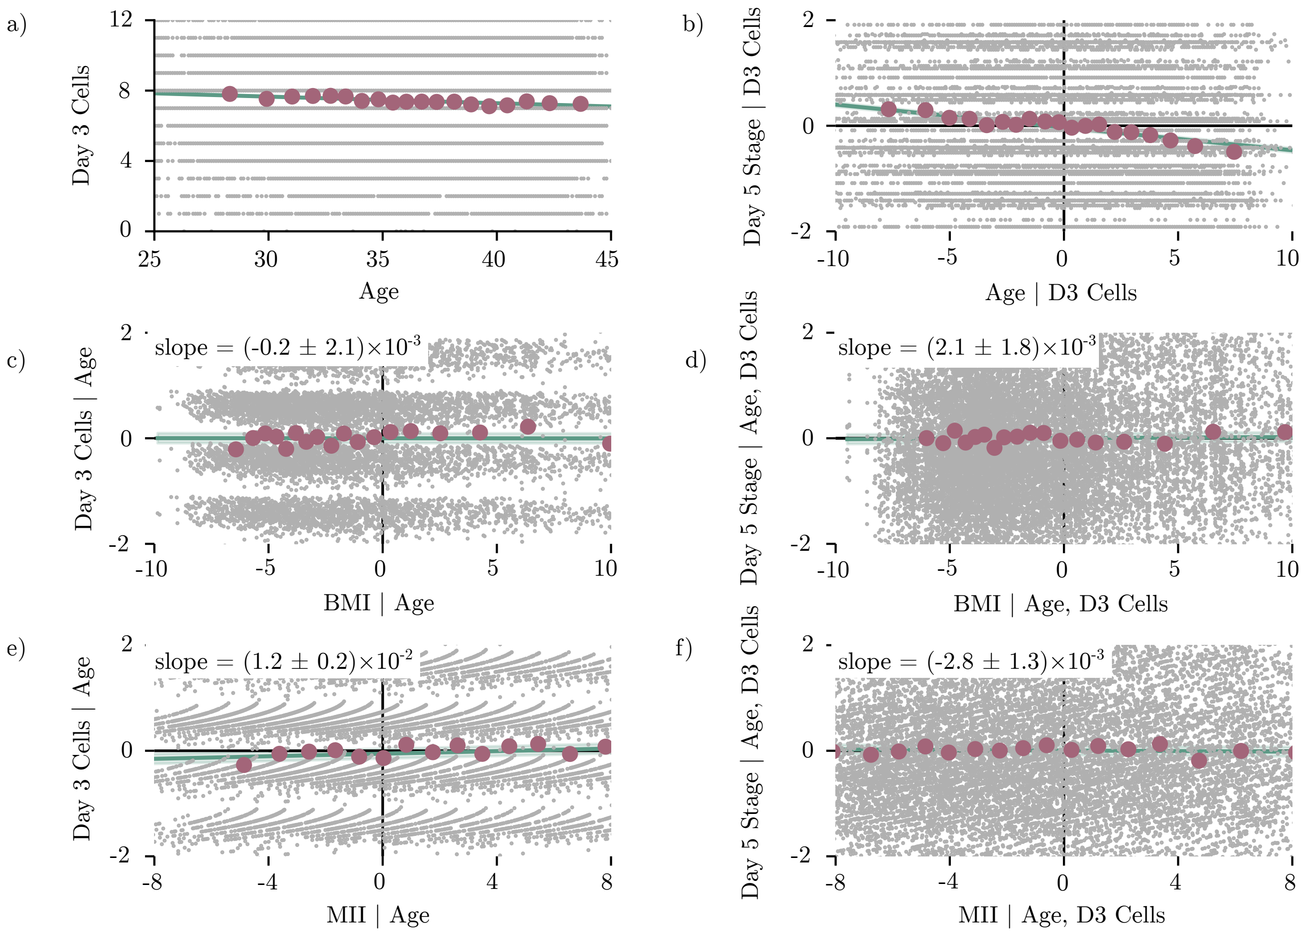


Figure 5: (a) Day 3 Cells vs Age. Green lines: linear fit to the data; red dots: data and standard error after grouping into 20 bins; gray dots: raw data. (b) Day 5 Stage vs Age, after regressing against Day 3 Cells. (c) Day 3 Cells vs BMI, after regressing against Age. The slope of the line is consistent with zero. (d) Day 5 Stage vs BMI, after regressing against Age and Day 3 Cells. The slope of the line is consistent with zero. (e) Day 3 Cells vs MII, after regressing against Age. The slope of the line is small but constrained away from zero. (f) Day 5 Stage vs MII, after regressing against Age and Day 3 Cells. The slope of the line is consistent with zero.

## 4.3 Embryonic Development

The data is consistent with neither BMI nor MII having any effect on the Day 5 stage of the embryo, after conditioning on Age and Day 3 Cells:

$$\text{Corr(BMI, Day 5 Stage} \mid \text{Age, Day 3 Cells)} = 0.007 \quad (P = 0.51)$$
$$\text{Corr(MII, Day 5 Stage} \mid \text{Age, Day 3 Cells)} = -0.011 \quad (P = 0.12)$$

However, the data paints a slightly more complex picture for the effect of BMI and MII on Day 3 Cells. The data is consistent with no correlation between BMI and Day 3 Cells, after conditioning on Age, but suggests a very weak but nonzero correlation between Day 3 Cells and MII.

$$\text{Corr(BMI, Day 3 Cells} \mid \text{Age, Day 3 Cells)} = -0.001 \quad (P = 0.94)$$
$$\text{Corr(MII, Day 3 Cells} \mid \text{Age, Day 3 Cells)} = 0.042 \quad (P = 1 \times 10^{-5})$$

While the measured correlation coefficient is nonzero between MII and Day 3 Cells (given Age), it is a tiny effect, as shown in SI Fig. 5e and as shown in Sec. 4.1, accounting for less than 0.2% of the variance in Day 3 Cells.

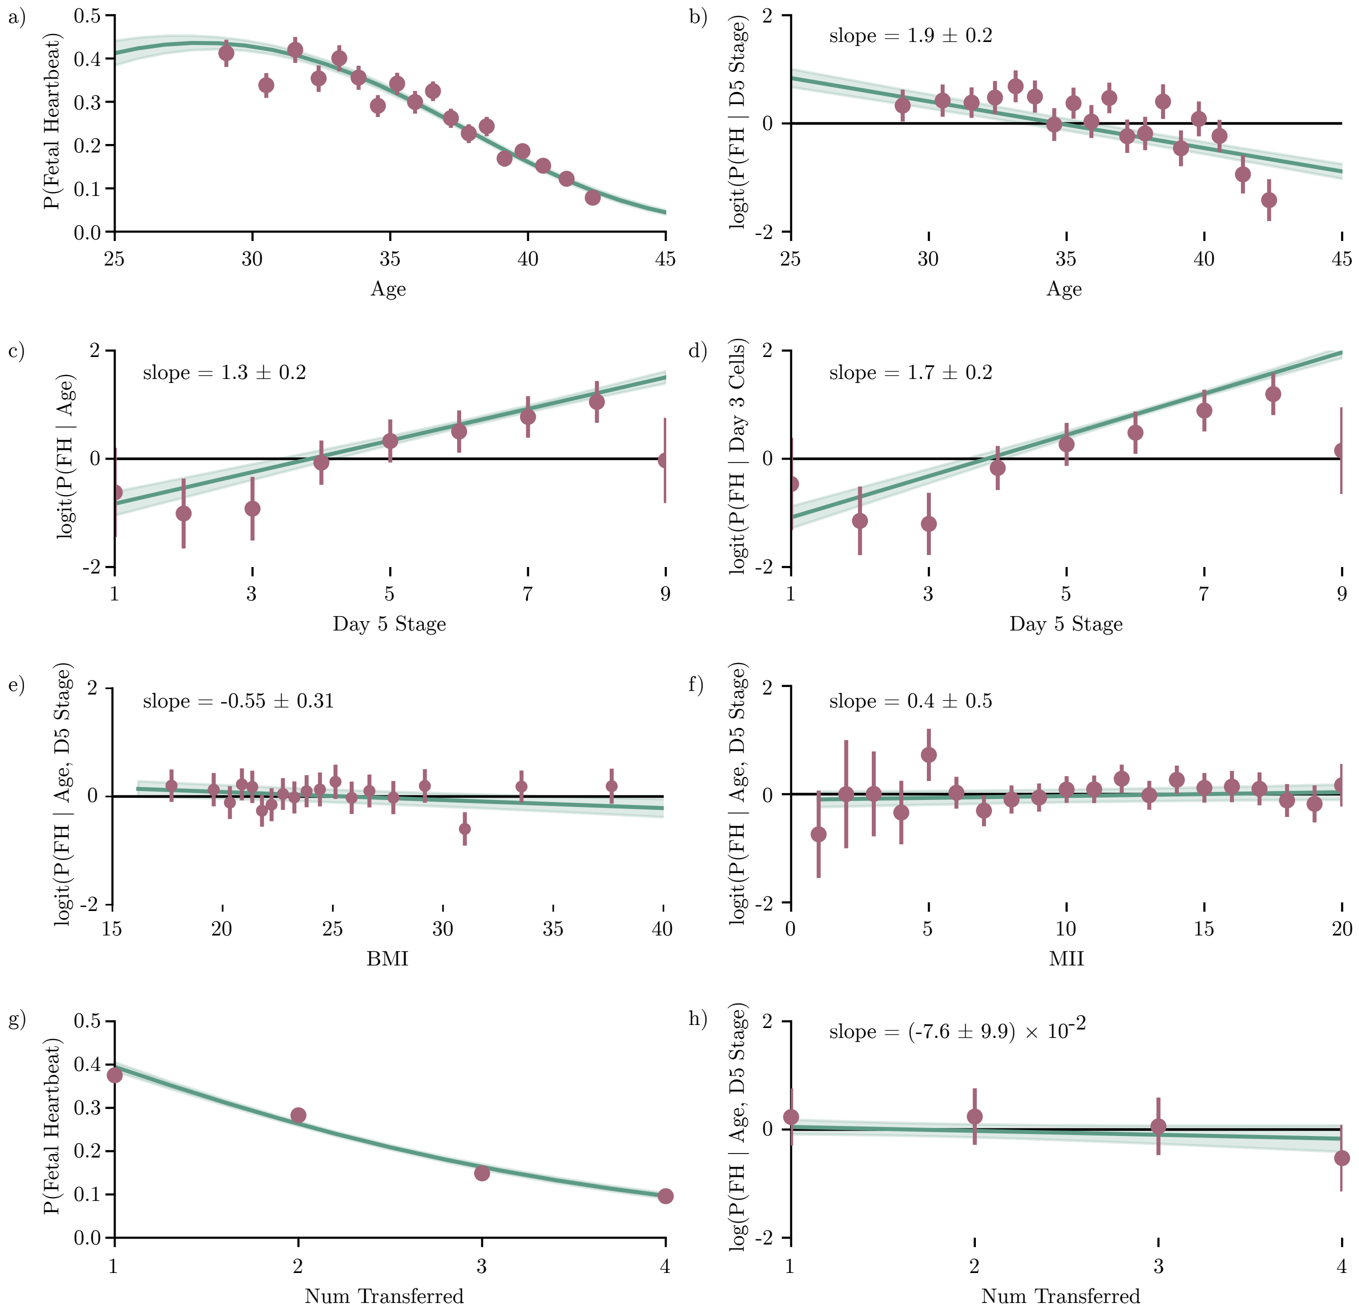


Figure 6: (a) Estimated probability of an embryo resulting in a fetal heartbeat (FH) as a function of Age alone. The red circles and errors show the probability estimated by a model that fits an independent probability of implantation for each number of cells; the green line and shaded region shows the nonlinear model with the highest model evidence and its error. (b) The logit of the estimated probability of FH as a function of Age, after regressing against Day 5 Stage. Red circles and error bars show the additional log probability estimated from a model that fits an independent logit for each value of Day 3 Cells; green line shows the best linear model for the logit and its uncertainty. Age is predictive of FH even after regressing on Day 5 Stage. (c) The logit of $P(\text{FH})$ vs Day 5 Stage, after regressing on Age. Day 5 Stage is predictive of FH even after regressing on Age. (d) The logit of $P(\text{FH})$ vs Day 5 Stage, after regressing on Day 3 Cells. Day 5 Stage is predictive of FH even after regressing on Day 3 Cells. (e) The logit of $P(\text{FH})$ vs BMI, after regressing on Age and Day 5 Stage. The data is consistent with BMI conferring no additional predictive on FH once Age and Day 5 Stage are known. (f) The logit of $P(\text{FH})$ vs MII, after regressing on Age and Day 5 Stage. The data is consistent with BMI conferring no additional predictive on FH once Age and Day 5 Stage are known. (g) Estimated probability of an embryo resulting in a fetal heartbeat as a function of the number of embryos transferred alone, and (h) the logit of $P(\text{FH})$ vs the number transferred, after regressing on Age and Day 5 Stage.

# References


[1] David JC MacKay and David JC Mac Kay. *Information theory, inference and learning algorithms.* Cambridge university press, 2003.

[2] Judea Pearl. *Causality.* Cambridge university press, 2009.

[3] Gideon Schwarz et al. Estimating the dimension of a model. *The annals of statistics*, 6(2):461–464, 1978.
